# Supplementary material for: Brain-on-Switch: Towards Advanced Intelligent Network Data Plane via NN-Driven Traffic Analysis at Line-Speed
Source: arXiv:2403.11090 source file (2024-03-17)
Supplement: Supplementary file 1 [file deprecated.tex]

From the first stage to the last in our workflow, the following components and operations are placed. 
Firstly, we place the flow management module, including the hash calculation for flow index and \textsf{TrueID}, and an array of register (called Register component in P4) to maintain the FlowInfo tuple (\ie {\textsf{TrueID}, timestamp}).

Then, we implement the embedding of raw features (\ie packet length and inter-packet delay (IPD)), taking $4$ stages in total: storage of timestamp of the last packet, calculation of IPD, embedding of IPD and packet length separately, and fully-connected layer of both packet length embedding and IPD embedding to output an embedding vector. 

The embedding vector is stored using $7$ bins (Registers) and dispatched to corresponding GRUs placed sequentially after this. 
The first two GRUs (\ie $\textsf{GRU}_{1,2}$) are merged into one match-action table, \ie $h'{=}\textsf{GRU}_2(\textsf{GRU}_1(0,ev_1),ev_2)$ is merged as $h'{=}(\textsf{GRU}_2\circ\textsf{GRU}_1)(0,ev_1,ev_2)$. 
The output layer is merged with GRU$_8$, \ie $C{=}\textsf{Output}(\textsf{GRU}_8(h,ev_8))$ is merged as $C{=}(\textsf{Output}\circ\textsf{GRU}_8)(h,ev_8)$. 

The counters (Registers) to accumulate per-class probabilities (CPR$_{1..8}$) are allocated immediately after the output layer. 
And then the \textsf{argmax} operation for $n{=}6,m{=}11$ is implemented. 
To overcome the limitation of TCAM resources, we split the \textsf{argmax} into two \textsf{argmax} operations for $n{=}3,m{=}11$ and one for $n{=}2,m{=}11$, as described in Figure \ref{fig:prototype}.
%To overcome the limitation of TCAM resources, we split the \textsf{argmax} into three \textsf{argmax} operations for $n{=}3,m{=}11$ and one for $n{=}2,m{=}11$, as described in \fixme{xxx}. 
Within the \textsf{argmax} operations, we subtract the maximum cumulative probability with the corresponding confidence threshold to check whether the confidence is strong or not.

Finally, the escalation logic is implemented. 
% We compare the maximum cumulative probability with the corresponding confidence threshold. 
If the confidence is weak, the counter (Register) for weak confidence result is updated. And if the counter exceeds the escalation threshold, we set the escalation flag (Register) of this flow.

In Tofino 1, there are not enough stages in ingress pipeline, so we leverage both the ingress and egress pipeline. 
The intermediate information is transferred from ingress to egress with bridged header. 
The problem is that the egress port should be determined in ingress pipeline, but we cannot determine whether a packet should be sent to \imis or not until the operations placed in egress are finished. 
To cope with this, We store the escalation flag in ingress pipeline to guide the decision of egress port and update the flag through egress-to-egress mirroring and recirculating.
%To cope with this, we place the result-based path selection in a second switch where the user-defined result-based processing logic of packet is implemented, or We can store the escalation flag in ingress pipeline to guide the decision of egress port and update the flag through egress-to-egress mirroring and recirculating.

%Another problem is that if the flows from different ingress pipelines can run to the same egress pipeline, the flow management should also be placed in egress, and even so, additional hash collisions can lead to storage waste in ingress pipelines. So we have to bind the ingress and egress pipeline one-to-one to avoid this problem. 

%Moreover, due to the limitation of the number of registers in a single stage, we have to place the bins of embedding vectors and the counters of cumulative probabilities in multiple stages.

The prototype costs nearly $23.4\%$ SRAM and less than $2\%$ TCAM and can be paralleled with applications mainly based on TCAM.
