# Supplementary material for: Brain-on-Switch: Towards Advanced Intelligent Network Data Plane via NN-Driven Traffic Analysis at Line-Speed
Source: arXiv:2403.11090 source file (2024-03-17)
Supplement: Supplementary file 2 [file deprecated_Select_The_Maximum_within_One_Stage.tex]

\section{Argmax With Ternary Matching}
%\section{Select The Maximum Within One Stage}
\label{sec:appendix_select_maximum}

The argmax operation, which is required in our online analysis, is not a primitive available on switch. The limitation of stages requires us to implement argmax within as less stages as possible and we implement argmax with ternary matching, as discussed in Section \ref{subsubsec:decision_making}.
%The limitation of stages requires us to select the maximum value within a single stage.
We define the problem as following conditions and restrictions.

\begin{enumerate}
\item There are $n$ numbers of $m$ bit(s) each, where $n,m\ge 1$.
\item There is a predefined order to determine which number to select when there is a tie for maximum value.
\item Only one ternary matching is allowed, i.e., the calculation before matching is prohibited.
\end{enumerate}

As discussed in Section \ref{subsubsec:decision_making}, We advance an algorithm to design the entries of ternary matching. Firstly, there are two base cases. For $n=1$, only one entry (i.e., all wildcards) is needed. For $m=1$, we need $n$ entries, i.e., enumerate the winning case of each number in predefined reverse order. For other cases, we start from the most significant bit (MSB), compare MSB of every number and (i) weed out the numbers whose MSB is smaller, or (ii) ignore the MSB when all numbers have the same MSB. Then the problem is reduced to a sub-problem with $m'=m-1$.
%We advance an algorithm to design the entries of ternary matching. Firstly, there are two base cases. For $n=1$, only one entry (i.e., all wildcards) is needed. For $m=1$, we need $n$ entries, i.e., enumerate the winning case of each number in predefined reverse order. For other cases, we first compare the most significant bits and (i) weed out some of the numbers, or (ii) ignore this bit when all bits are equal. Then the problem is reduced to a sub-problem with $m'=m-1$.

We denote the number of required entries based on our algorithm as $F(n,m)$. The recurrence relations of $F$ is given as follows.

\begin{equation}
\label{math:base,m=1}
F(n,1)=n,n\ge 1
\end{equation}

\begin{equation}
\label{math:base,n=1}
F(1,m)=1,m\ge 1
\end{equation}

\begin{equation}
\label{math:recursion}
F(n,m)=F(n,m-1)+\sum_{i=1}^{n-1}\binom{n}{i}F(i,m-1),n\ge 2,m\ge 2
\end{equation}

The meaning of \ref{math:recursion} is described as follows. If there are $i$ numbers whose most significant bit (MSB) is 1 ($i\in [1,n-1]$), similar as the case $\mathcal{C}_{(l,i)}$ defined in Section \ref{subsubsec:decision_making}, then we only have to focus on the comparison of these $i$ numbers with the rest $m-1$ bits, of which the number of entries is $F(i,m-1)$ and there are $\binom{n}{i}$ possible cases for which $i$ numbers have $\textsf{MSB=1}$. Otherwise, the MSBs are all the same (\ie the case $\mathcal{C}_{(l,n)}$ and $\mathcal{C}_{(l,0)}$ defined in Section \ref{subsubsec:decision_making}), and the number of entries is $F(n,m-1)$.

%The meaning of \ref{math:recursion} is described as follows. If there are $i$ numbers whose most significant bit is '1',  then we only have to focus on these $i$ numbers, ignoring the rest $n-i$ numbers (i.e., using wildcard). Otherwise, the most significant bits are all the same, and we ignore this bit (i.e., using wildcard) and continue with the rest $m-1$ bits for each number.

The conclusion is that $F(n,m)=nm^{n-1}$. The simplest way to verify it is the mathematical induction. 

\begin{equation}
\begin{aligned}
F(n,m-1)+\sum_{i=1}^{n-1}\binom{n}{i}F(i,m-1)\\
=\sum_{i=1}^{n}\binom{n}{i}i(m-1)^{i-1}\\
=n\sum_{i=1}^{n}\binom{n-1}{i-1}(m-1)^{i-1}\\
=n\sum_{i=0}^{n-1}\binom{n-1}{i}(m-1)^{i}\\
=nm^{n-1}=F(n,m)
\end{aligned}
\end{equation}

We give another derivation process from the equation \ref{math:recursion} as follows. Firstly, let $F(0,m)=0,m\ge 1$, which is 
consistent with the equation \ref{math:base,m=1}. Then the equation \ref{math:recursion} can be written as below.

\begin{equation}
F(n,m)=\sum_{i=0}^{n}\binom{n}{i}F(i,m-1),n\ge 0,m\ge 2
\end{equation}

We transform the formula and get:
\begin{equation}
F(n,m)=\sum_{i=0}^{n}\frac{n!}{i!(n-i)!}F(i,m-1),n\ge 0,m\ge 2
\end{equation}

\begin{equation}
\label{math:deformation}
\frac{F(n,m)}{n!}=\sum_{i=0}^{n}\frac{F(i,m-1)}{i!}\frac{1}{(n-i)!},n\ge 0,m\ge 2
\end{equation}

We denote $\frac{F(n,m)}{n!}$ as $^{m}g_n$, and $\frac{1}{n!}$ as $h_n$. Then we construct the generating function of $^{m}g$ and $h$.

\begin{equation}
\label{math:generation,g}
^{m}G(x)=\sum_{n=0} {^{m}g_{n}}x^n=\sum_{n=0}\frac{F(n,m)}{n!}x^n,m\ge 1
\end{equation}

\begin{equation}
H(x)=\sum_{n=0}h_{n}x^n=\sum_{n=0}\frac{x^n}{n!}=e^x
\end{equation}

We can obtain the recursive relations between $^{m}G$ and $^{m-1}G$ from equation \ref{math:deformation}.

\begin{equation}
^{m}G=^{m-1}G\times H,m\ge 2
\end{equation}

And for $m=1$, we have

\begin{equation}
\begin{aligned}
^{1}G(x)=\sum_{n=0} {^{1}g_{n}}x^n=\sum_{n=0}\frac{F(n,1)}{n!}x^n\\
=\sum_{n=0}\frac{n}{n!}x^n=\sum_{n=1}\frac{1}{(n-1)!}x^n\\
=x\sum_{n=0}\frac{1}{n!}x^n=xe^x
\end{aligned}
\end{equation}

With the mathematical induction, we can get

\begin{equation}
^{m}G(x)=xe^{mx},m\ge 1
\end{equation}

Compared with the equation \ref{math:generation,g} and we can get

\begin{equation}
\begin{aligned}
F(n,m)=^{m}G^{(n)}(0)=(x e^{m x})^{(n)}\bigg|_{x=0}\\
=(n m^{n-1}+m^n x)e^{m x}\bigg|_{x=0}\\
=nm^{n-1},n\ge 1,m\ge 1
\end{aligned}
\end{equation}

QED.
